# Supplementary material for: Towards a Transpiler for C/C++ to Safer Rust
Source: arXiv:2401.08264 source file (2024-01-16)
Supplement: Supplementary file 1 [file at_examples.tex]

\section{Examples considered for analysis of the existing automatic transpilers}
\label{appendix:examples}
\subsection{C Language}
\label{appendix1:eg}
\begin{enumerate}
	\item Recursive Fibonacci Numbers

		\begin{figure}[hbt!]
	\begin{lstlisting}[style=ES6][autogobble]
		// Fibonacci Series using Recursion
		#include <stdio.h>
		int fib(int n)
		{
			if (n <= 1)
			return n;
			return fib(n - 1) + fib(n - 2);
		}
		
		int main()
		{
			int n = 9;
			printf("%d", fib(n));
			getchar();
			return 0;
		}
		
	\end{lstlisting}
	\caption{Recursive Fibonacci Numbers in C}
\end{figure}
\FloatBarrier

\item Linked List Implementation

\begin{figure}[hbt!]
	\begin{lstlisting}[style=ES6][autogobble]
		// A simple C program for
		// traversal of a linked list
		
		#include <stdio.h>
		#include <stdlib.h>
		
		struct Node {
			int data;
			struct Node* next;
		};
		
		// This function prints contents of linked list starting
		// from the given node
		void printList(struct Node* n)
		{
			while (n != NULL) {
				printf(" %d ", n->data);
				n = n->next;
			}
		}
		
		// Driver's code
		int main()
		{
			struct Node* head = NULL;
			struct Node* second = NULL;
			struct Node* third = NULL;
			
			// allocate 3 nodes in the heap
			head = (struct Node*)malloc(sizeof(struct Node));
			second = (struct Node*)malloc(sizeof(struct Node));
			third = (struct Node*)malloc(sizeof(struct Node));
			
			head->data = 1; // assign data in first node
			head->next = second; // Link first node with second
			
			second->data = 2; // assign data to second node
			second->next = third;
			
			third->data = 3; // assign data to third node
			third->next = NULL;
			
			// Function call
			printList(head);
			
			return 0;
		}
		
	\end{lstlisting}
	\caption{Linked List Implementation in C}
\end{figure}
\FloatBarrier
\end{enumerate}

\subsection{C++ Language}
\label{appendix2:eg}
\begin{enumerate}
	\item Catalan Numbers
	
	\begin{figure}[hbt!]
		\begin{lstlisting}[style=ES6][autogobble]
		#include <iostream>
		using namespace std;
		
		// A recursive function to find nth catalan number
		unsigned long int catalan(unsigned int n)
		{
			// Base case
			if (n <= 1)
			return 1;
			
			// catalan(n) is sum of
			// catalan(i)*catalan(n-i-1)
			unsigned long int res = 0;
			for (int i = 0; i < n; i++)
			res += catalan(i) * catalan(n - i - 1);
			
			return res;
		}
		
		// Driver code
		int main()
		{
			for (int i = 0; i < 10; i++)
			cout << catalan(i) << " ";
			return 0;
		}

		\end{lstlisting}
		\caption{Catalan Numbers in C++}
	\end{figure}
	\FloatBarrier

	\item Basic OOPS in C++

	\begin{figure}[hbt!]
		\begin{lstlisting}[style=ES6][autogobble]
		// C++ program to demonstrate constructors
		
		#include <bits/stdc++.h>
		using namespace std;
		class Geeks
		{
			public:
			int id;
			
			//Default Constructor
			Geeks()
			{
				cout << "Default Constructor called" << endl;
				id=-1;
			}
			
			//Parameterized Constructor
			Geeks(int x)
			{
				cout <<"Parameterized Constructor called "<< endl;
				id=x;
			}
		};
		int main() {
			
			// obj1 will call Default Constructor
			Geeks obj1;
			cout <<"Geek id is: "<<obj1.id << endl;
			
			// obj2 will call Parameterized Constructor
			Geeks obj2(21);
			cout <<"Geek id is: " <<obj2.id << endl;
			return 0;
		}

		\end{lstlisting}
		\caption{C++ program to demonstrate constructors}
	\end{figure}
	\FloatBarrier
\end{enumerate}
