# Supplementary material for: Towards a Transpiler for C/C++ to Safer Rust
Source: arXiv:2401.08264 source file (2024-01-16)
Supplement: Supplementary file 2 [file at_results.tex]

\section{Automatic Transpilation Results}
\label{appendix:results}
\subsection{C2Rust}
\begin{figure}[hbt!]
	\begin{lstlisting}[style=ES6]
		#![allow(dead_code, mutable_transmutes, non_camel_case_types, non_snake_case,
		non_upper_case_globals, unused_assignments, unused_mut)]
		#![register_tool(c2rust)]
		#![feature(main, register_tool)]
		extern "C" {
			#[no_mangle]
			fn getchar() -> libc::c_int;
			#[no_mangle]
			fn printf(_: *const libc::c_char, _: ...) -> libc::c_int;
		}
		//Fibonacci Series using Recursion
		#[no_mangle]
		pub unsafe extern "C" fn fib(mut n: libc::c_int) -> libc::c_int {
			if n <= 1 as libc::c_int { return n }
			return fib(n - 1 as libc::c_int) + fib(n - 2 as libc::c_int);
		}
		unsafe fn main_0() -> libc::c_int {
			let mut n: libc::c_int = 9 as libc::c_int;
			printf(b"%d\x00" as *const u8 as *const libc::c_char, fib(n));
			getchar();
			return 0 as libc::c_int;
		}
		#[main]
		pub fn main() { unsafe { ::std::process::exit(main_0() as i32) } }
	\end{lstlisting}
	\caption{C2Rust Transpilation: Recursive Fibonacci}
\end{figure}
\FloatBarrier

\begin{figure}[hbt!]
	\begin{lstlisting}[style=ES6][frame=single,autogobble,basicstyle=\scriptsize\ttfamily][label={lst:firstLst},caption={The first listing}]
		#![allow(dead_code, mutable_transmutes, non_camel_case_types, non_snake_case,
		non_upper_case_globals, unused_assignments, unused_mut)]
		#![register_tool(c2rust)]
		#![feature(main, register_tool)]
		extern "C" {
			#[no_mangle]
			fn printf(_: *const libc::c_char, _: ...) -> libc::c_int;
			#[no_mangle]
			fn malloc(_: libc::c_ulong) -> *mut libc::c_void;
		}
		// A simple C program for traversal of a linked list
		#[derive(Copy, Clone)]
		#[repr(C)]
		pub struct Node {
			pub data: libc::c_int,
			pub next: *mut Node,
		}
		// This function prints contents of linked list starting from
		// the given node
		#[no_mangle]
		pub unsafe extern "C" fn printList(mut n: *mut Node) {
			while !n.is_null() {
				printf(b" %d \x00" as *const u8 as *const libc::c_char, (*n).data);
				n = (*n).next
			};
		}
		unsafe fn main_0() -> libc::c_int {
			let mut head: *mut Node = 0 as *mut Node;
			let mut second: *mut Node = 0 as *mut Node;
			let mut third: *mut Node = 0 as *mut Node;
			// allocate 3 nodes in the heap
			head =
			malloc(::std::mem::size_of::<Node>() as libc::c_ulong) as
			*mut Node; // assign data in first node
			second =
			malloc(::std::mem::size_of::<Node>() as libc::c_ulong) as
			*mut Node; // Link first node with second
			third =
			malloc(::std::mem::size_of::<Node>() as libc::c_ulong) as
			*mut Node; // assign data to second node
			(*head).data = 1 as libc::c_int; // assign data to third node
			(*head).next = second;
			(*second).data = 2 as libc::c_int;
			(*second).next = third;
			(*third).data = 3 as libc::c_int;
			(*third).next = 0 as *mut Node;
			printList(head);
			return 0 as libc::c_int;
		}
		#[main]
		pub fn main() { unsafe { ::std::process::exit(main_0() as i32) } }
	\end{lstlisting}
	\caption{C2Rust Transpilation: Linked List Implementation in C}
\end{figure}

\begin{figure}[hbt!]
	\begin{lstlisting}[style=ES6]
		#![allow(dead_code, mutable_transmutes, non_camel_case_types, non_snake_case,
		non_upper_case_globals, unused_assignments, unused_mut)]
		#![register_tool(c2rust)]
		#![feature(main, register_tool)]
		#[no_mangle]
		pub static mut namespace: libc::c_int = 0;
		// A recursive function to find nth catalan number
		#[no_mangle]
		pub unsafe extern "C" fn catalan(mut n: libc::c_uint) -> libc::c_ulong {
			// Base case
			if n <= 1 as libc::c_int as libc::c_uint {
				return 1 as libc::c_int as libc::c_ulong
			}
			// catalan(n) is sum of
			// catalan(i)*catalan(n-i-1)
			let mut res: libc::c_ulong = 0 as libc::c_int as libc::c_ulong;
			let mut i: libc::c_int = 0 as libc::c_int;
			while (i as libc::c_uint) < n {
				res =
				res.wrapping_add(catalan(i as
				libc::c_uint).wrapping_mul(catalan(n.wrapping_sub(i
				as
				libc::c_uint).wrapping_sub(1
				as
				libc::c_int
				as
				libc::c_uint))));
				i += 1
			}
			return res;
		}
		// Driver code
		unsafe fn main_0() -> libc::c_int { return 0 as libc::c_int; }
		#[main]
		pub fn main() { unsafe { ::std::process::exit(main_0() as i32) } }
	\end{lstlisting}
	\caption{C2Rust Transpilation: Catalan Numbers}
\end{figure}
\FloatBarrier

\begin{figure}[hbt!]
	\begin{lstlisting}[style=ES6]
		#![allow(dead_code, mutable_transmutes, non_camel_case_types, non_snake_case,
		non_upper_case_globals, unused_assignments, unused_mut)]
		#![register_tool(c2rust)]
		#![feature(main, register_tool)]
		// C++ program to demonstrate constructors
		#[no_mangle]
		pub static mut namespace: libc::c_int = 0;
		#[no_mangle]
		pub static mut Geeks: libc::c_int = 0;
		//Default Constructor
		//Parameterized Constructor
		unsafe fn main_0() -> libc::c_int {
			// obj1 will call Default Constructor
			// obj2 will call Parameterized Constructor
			return 0 as libc::c_int;
		}
		#[main]
		pub fn main() { unsafe { ::std::process::exit(main_0() as i32) } }
	\end{lstlisting}
	\caption{C2Rust Transpilation: Basic OOPs}
\end{figure}
\FloatBarrier

\clearpage

\subsection{CRust}
\begin{figure}[hbt!]
	\begin{lstlisting}[style=ES6]
		/*************************************************************************
		* This file was generated by CRUST by an automated semantics preserving
		* translation from C/C++ to Rust
		* CRUST isn't perfect and may require manual editing
		* Check warnings and errors and refer to the official Rust Documentation
		************************************************************************/
		
		/** Crust doesn't resolve C/C++ dependencies or included header.
		* You may have to define your own module and implement those functionality in Rust
		* Or you can translate header file with Crust to produce Rust code. *
		* >>>>>>>> # include < bits / stdc ++ . h >
		**/
		//FIXME: Convert the below statement manually,
		/**
		using namespace std ;
		*/
		fn fib(n: i32) -> i32 {
			if (n <= 1) == true {
				/** Crust tries to identify return statement and replace with rust equivalent
				* shorthand notation. If error found in this line, Please replace shorthand notation
				* with return statement
				**/
				n
			}
			/** Crust tries to identify return statement and replace with rust equivalent
			* shorthand notation. If error found in this line, Please replace shorthand notation
			* with return statement
			**/
			return fib(n - 1) + fib(n - 2);
		}
		fn main() {
			/*Crust with Strict Mode enabled, declares all variables as immutable.
			* If you are mutating the below variable anywhere in program, please change the declaration statement as
			* let mut var_name:type=init_val;
			**/
			let n: i32 = 9;
			printf("%d\n", fib(n));
			getchar();
			/** Crust tries to identify return statement and replace with rust equivalent
			* shorthand notation. If error found in this line, Please replace shorthand notation
			* with return statement
			**/
			return 0;
		}
	\end{lstlisting}
	\caption{CRust Transpilation: Recursive Fibonacci}
\end{figure}

\begin{figure}[hbt!]
	\begin{lstlisting}[style=ES6]
		/*************************************************************************
		* This file was generated by CRUST by an automated semantics preserving
		* translation from C/C++ to Rust
		* CRUST isn't perfect and may require manual editing
		* Check warnings and errors and refer to the official Rust Documentation
		************************************************************************/
		// C program to implement a
		// linked list
		
		/** Crust doesn't resolve C/C++ dependencies or included header.
		* You may have to define your own module and implement those functionality in Rust 
		* Or you can translate header file with Crust to produce Rust code. * 
		* >>>>>>>> # include < stdio . h >
		**/
		* >>>>>>>> # include < stdlib . h >
		**/
		
		
		
		/** Declaration of a structure should be completed with initialization of it's fields
		* It should be in the following format
		* let variable:struct_name = struct_name { member1:value1, member2:value2,..}
		*/ let 
		= Node { }; 
		
		/** Declaration of a structure should be completed with initialization of it's fields
		* It should be in the following format
		* let variable:struct_name = struct_name { member1:value1, member2:value2,..}
		*/ let * = Node { }; 
		; 
		
		// Driver's code
		fn main ( ) { 
			
			/** Declaration of a structure should be completed with initialization of it's fields
			* It should be in the following format
			* let variable:struct_name = struct_name { member1:value1, member2:value2,..}
			*/ let * = Node { }; 
			
			/** Declaration of a structure should be completed with initialization of it's fields
			* It should be in the following format
			* let variable:struct_name = struct_name { member1:value1, member2:value2,..}
			*/ let * = Node { }; 
			
			/** Declaration of a structure should be completed with initialization of it's fields
			* It should be in the following format
			* let variable:struct_name = struct_name { member1:value1, member2:value2,..}
		\end{lstlisting}
	\end{figure}
	
	\begin{figure}[hbt!]
		\begin{lstlisting}[style=ES6]
			*/ let * = Node { }; 
			
			// allocate 3 nodes in the heap
			head = ( ; 
			second = ( ; 
			third = ( ; 
			
			
			head . data = 1 ; // assign data in first node
			head . next = second ; // Link first node with
			// the second node
			
		\end{lstlisting}
	\end{figure}
	
	\begin{figure}[hbt!]
		\begin{lstlisting}[style=ES6]
			// assign data to second node
			second . data = 2 ; 
			
			// Link second node with the third node
			second . next = third ; 
			
			third . data = 3 ; // assign data to third node
			third . next = NULL ; 
			
			
			/** Crust tries to identify return statement and replace with rust equivalent
			* shorthand notation. If error found in this line, Please replace shorthand notation 
			* with return statement 
			**/
			return 0 ; 
		}
	\end{lstlisting}
	\caption{CRust Transpilation: Linked List Implementation in C}
\end{figure}
\FloatBarrier

\begin{figure}[hbt!]
	\begin{lstlisting}[style=ES6]
		/*************************************************************************
		* This file was generated by CRUST by an automated semantics preserving
		* translation from C/C++ to Rust
		* CRUST isn't perfect and may require manual editing
		* Check warnings and errors and refer to the official Rust Documentation
		************************************************************************/
		
		/*Crust with Strict Mode enabled, declares all variables as immutable.
		* If you are mutating the below variable anywhere in program, please change the declaration statement as
		* let mut var_name:type=init_val;
		**/
		static n : i64 ;
		
		// catalan(n) is sum of
		// catalan(i)*catalan(n-i-1)
		
		/*Crust with Strict Mode enabled, declares all variables as immutable.
		* If you are mutating the below variable anywhere in program, please change the declaration statement as
		* let mut var_name:type=init_val;
		**/
		static res : i64 = 0; ;
		
		/*Crust with Strict Mode enabled, declares all variables as immutable.
		* If you are mutating the below variable anywhere in program, please change the declaration statement as
		* let mut var_name:type=init_val;
		**/
		static i : i32 = 0; ; while i < n {
			res += catalan ( i ) * catalan ( n - i - 1 ) ; i +=1 ; }
	\end{lstlisting}
	\caption{C2Rust Transpilation: Catalan Numbers}
\end{figure}
\FloatBarrier
