# Supplementary material for: Towards a Transpiler for C/C++ to Safer Rust
Source: arXiv:2401.08264 source file (2024-01-16)
Supplement: Supplementary file 3 [file man_results.tex]

\section{Manual Transpilation Result}
\label{appendix:result}
\subsection{Tizen's gperf module's Bool-Array file Transpilation from C++ to Rust}
\begin{figure}[hbt!]
	\begin{lstlisting}[style=ES6]
		#ifndef bool_array_h
		#define bool_array_h 1
		
		/* A Bool_Array instance is a bit array of fixed size, optimized for being
		filled sparsely and cleared frequently.  For example, when processing
		tests/chill.gperf, the array will be:
		- of size 15391,
		- clear will be called 3509 times,
		- set_bit will be called 300394 times.
		With a conventional bit array implementation, clear would be too slow.
		With a tree/hash based bit array implementation, set_bit would be slower. */
		
		class Bool_Array
		{
			public:
			/* Initializes the bit array with room for SIZE bits, numbered from
			0 to SIZE-1. */
			Bool_Array (unsigned int size);
			
			/* Frees this object.  */
			~Bool_Array ();
			
			/* Resets all bits to zero.  */
			void                  clear ();
			
			/* Sets the specified bit to true.
			Returns its previous value (false or true).  */
			bool                  set_bit (unsigned int index);
			
			private:
			/* Size of array.  */
			unsigned int const    _size;
			
			/* Current iteration number.  Always nonzero.  Starts out as 1, and is
			incremented each time clear() is called.  */
			unsigned int          _iteration_number;
			
			/* For each index, we store in storage_array[index] the iteration_number at
			the time set_bit(index) was last called.  */
			unsigned int * const  _storage_array;
		};
		
		#ifdef __OPTIMIZE__  /* efficiency hack! */
		
		#include <stdio.h>
		#include <string.h>
		#include "options.h"
		#define INLINE inline
		#include "bool-array.icc"
		#undef INLINE
		
		#endif
		
		#endif\end{lstlisting}
	\caption{bool-array.h file}
\end{figure}
\FloatBarrier

\begin{figure}[hbt!]			
	\begin{lstlisting}[style=ES6][frame=single,autogobble,basicstyle=\scriptsize\ttfamily][label={lst:firstLst},caption={The first listing}]
		/* Initializes the bit array with room for SIZE bits, numbered from
		0 to SIZE-1. */
		INLINE
		Bool_Array::Bool_Array (unsigned int size)
		: _size (size),
		_iteration_number (1),
		_storage_array (new unsigned int [size])
		{
			memset (_storage_array, 0, size * sizeof (_storage_array[0]));
			if (option[DEBUG])
			fprintf (stderr, "\nbool array size = %d, total bytes = %d\n",
			_size,
			static_cast<unsigned int> (_size * sizeof (_storage_array[0])));
		}
		
		/* Sets the specified bit to true.
		Returns its previous value (false or true).  */
		INLINE bool
		Bool_Array::set_bit (unsigned int index)
		{
			if (_storage_array[index] == _iteration_number)
			/* The bit was set since the last clear() call.  */
			return true;
			else
			{
				/* The last operation on this bit was clear().  Set it now.  */
				_storage_array[index] = _iteration_number;
				return false;
			}
		}
		
		/* Resets all bits to zero.  */
		INLINE void
		Bool_Array::clear ()
		{
			/* If we wrap around it's time to zero things out again!  However, this only
			occurs once about every 2^32 iterations, so it will not happen more
			frequently than once per second.  */
			
			if (++_iteration_number == 0)
			{
				_iteration_number = 1;
				memset (_storage_array, 0, _size * sizeof (_storage_array[0]));
				if (option[DEBUG])
				{
					fprintf (stderr, "(re-initialized bool_array)\n");
					fflush (stderr);
				}
			}
		}
	\end{lstlisting}
	\caption{bool-array.icc file}
\end{figure}

\begin{figure}[hbt!]
	\begin{lstlisting}[style=ES6]
		/* Specification. */
		#include "bool-array.h"
		
		#include <stdio.h>
		#include <string.h>
		#include "options.h"
		
		/* Frees this object.  */
		Bool_Array::~Bool_Array ()
		{
			/* Print out debugging diagnostics. */
			if (option[DEBUG])
			fprintf (stderr, "\ndumping boolean array information\n"
			"size = %d\niteration number = %d\nend of array dump\n",
			_size, _iteration_number);
			delete[] const_cast<unsigned int *>(_storage_array);
		}
		
		#ifndef __OPTIMIZE__
		
		#define INLINE /* not inline */
		#include "bool-array.icc"
		#undef INLINE
		
		#endif /* not defined __OPTIMIZE__ */\end{lstlisting}
	\caption{bool-array.cc file}
\end{figure}
\FloatBarrier

\begin{figure}[hbt!]
	\begin{lstlisting}[style=ES6]
		pub struct Bool_Array
		{
			_size: u32,
			_iteration_number: u32,
			_storage_array: Vec<u32>,
		}
		
		impl Bool_Array {
			pub fn new(size: u32) -> Bool_Array {
				Bool_Array{
					_size : size,
					_iteration_number : 0,
					_storage_array : vec![0; size as usize],
				}
				
				// implement the print after doing options file
			}
			
			#[inline]
			pub fn set_bit(&mut self, index: u32) -> bool {
				if self._storage_array[index as usize] == self._iteration_number
				{
					return true;
				}
				else
				{
					self._storage_array[index as usize] = self._iteration_number;
					return false;
				}
			}
			
			#[inline]
			pub fn clear(&mut self) {
				self._iteration_number += 1;
				
				if self._iteration_number == 0
				{
					self._iteration_number = 1;
					self._storage_array = vec![0; self._size as usize];
				}
			}
	}\end{lstlisting}
	\caption{bool-array.rs file: Rust file obtained from manually transpiling bool-array C++ files to Rust}
\end{figure}
\FloatBarrier
