# Supplementary material for: Towards a Transpiler for C/C++ to Safer Rust
Source: arXiv:2401.08264 source file (2024-01-16)
Supplement: Supplementary file 4 [file Appendix.pdf]

# Towards a Transpiler from C/C++ to Safer Rust

## *Appendix Contents*

### **Appendix A: Error Handling using Result Enum**

The *Result* type is a generic enumeration provided by the Rust standard library. It represents the result of a computation that can either be successful (*Ok* variant) or unsuccessful (*Err* variant).

In the example code shown in Figure A1, the *parse\_int* function tries to parse an integer from a string. If the parsing is successful, the function returns an *Ok* variant containing the parsed integer. If the parsing fails, the function returns an *Err* variant containing the *ParseIntError* that occurred.

```
fn parse_int(s: &str) -> Result<i32, std::num::ParseIntError> {
    s.parse::<i32>().map_err(|e| e.into())
}

fn main() {
    let result = parse_int("5");
    match result {
        Ok(n) => println!("Parsed integer: {}", n),
        Err(e) => println!("Error parsing integer: {}", e),
    }
}
```

**Figure A1.** Result Enum usage in Rust

Pattern matching can be used to handle the *Result* value. In example A1, match expression is used to handle the *Ok* and *Err* variants. The *unwrap* method can also be used to extract the value from an *Ok* variant, but this will panic if the value is an *Err* variant, as shown in Figure A2.

```
let result = parse_int("5");
let n = result.unwrap(); // Will panic if result is an Err variant
println!("Parsed integer: {}", n);
```

**Figure A2.** Result Enum usage in Rust

Hence, it is not recommended to use *unwrap()* in production code due to the possibility of panic. *map* and *map\_err* methods are other ways to handle a *Result* value which allow us to transform the value inside the *Ok* or *Err* variant by applying a function to it.

## **Appendix B: Borrowing and Rules of Borrowing in Rust**

It is allowed in Rust to borrow a value, which grants temporary access to the variable. Instead of taking variables as arguments in functions, references of the variables are taken as arguments. This way, ownership of the resource is borrowed rather than owned.

```
fn main() {  
    // Borrow vector and return the sum of its elements.  
    fn sum_vec(v: &Vec<i32>) -> i32 {  
        // Do stuff with `v`.  
        let mut sum = 0;  
        for num in v.iter() {  
            sum += num;  
        }  
        // Return the answer.  
        sum  
    }  
    let v = vec![1, 2, 3];  
    let answer = sum_vec(&v);  
    println!("{}", answer);  
}
```

**Figure B1.** Example of borrowing in Rust

In Figure B1, a function named **sum\_vec** is defined, which receives a reference to a vector of *i32* integers as an input argument and returns the sum of its elements. The function uses the **&** symbol to indicate that it borrows the vector instead of taking ownership of it.

Rather than accepting **Vec<i32>** as its argument, the function takes a reference: **&Vec<i32>**. Thus, instead of passing the vector **v** directly, a reference to it is passed using **&v**. The type **&T** is called a "reference" and, unlike owning the resource, borrows ownership. A binding that borrows something does not deallocate the resource when it goes out of scope. Consequently, after the call to **sum\_vec()**, the original bindings can be used again.

## B.1: Immutable Borrows

```
fn main() {
    fn foo(v: &Vec<i32>) {
        v.push(5);
    }
    let v = vec![];
    foo(&v);
}
/* error: cannot borrow immutable borrowed content `*v` as mutable
v.push(5);    */
```

**Figure B2.** Example of immutable borrows in Rust

Figure B2 defines a function called *foo* that takes a reference to a vector of *i32* integers as its argument. Within the function, it attempts to push the value *5* onto the vector. References are immutable, like bindings. This means that inside *foo()*, the vectors cannot be changed at all. In the *main* function, a new vector *v* is created and initialized to an empty vector. The *foo* function is called with a reference to *v* as its argument. After the call to *foo*, there is an attempt to push the value *5* onto the vector *v*. However, this results in a compile-time error because the function *foo* borrowed the vector as immutable, which means that it cannot be mutated within the *foo* function.

## B.2: Mutable Borrows

In some cases, a borrowed value may need to be modified, which can be achieved through the use of a mutable borrow. A second type of reference, known as a 'mutable reference', permits the resource being borrowed to be mutated.

```
fn main() {
    fn foo(v: &mut Vec<i32>) {
        v.push(5);
    }
    let mut v = vec![2];
    foo(&mut v);
    println!("v[1] is: {}", v[1]);
}
```

**Figure B3.** Example of mutable borrows in Rust

In Figure B3, the code defines a function *foo* that takes a mutable reference to a vector of *i32*, appends the integer *5* to it. In the *main* function, a vector of *i32* integers *v* is defined

and initialized with the value of **2**. Then the *foo* function is called with a mutable reference to the vector *&mut v*, which allows the function to modify the contents of the vector. Finally, it prints out the value of the second element of the modified vector *v* which is **5**.

### **B.3: Rules of Borrowing**

In Rust, borrowing rules state that a borrow must not outlast its owner's scope, and only one mutable reference or one or more references to a resource can exist at a time. These rules prevent data races by ensuring that multiple pointers cannot access the same memory location at the same time, with at least one of them writing, without synchronization.

```
fn main() {  
    let mut v = vec![2];  
    let v2 = &v;  
    let v3 = &v;  
    let v4 = &mut v;  
    println!("{}", v2[0], v3[0], v4[0]);  
}  
/* cannot borrow `v` as mutable because it is also borrowed as immutable*/
```

**Figure B4.** Example of single mutable borrow feature in Rust

Figure B4 shows a Rust program that creates a mutable vector *v* containing two integers, **[2, 6]**. It then creates two immutable references to *v*, *v2* and *v3*, and one mutable reference to *v*, *v4*. Finally, the program attempts to print the first element of each reference, which would be **2, 2, and 2**, respectively.

However, the code results in a compile-time error: "cannot borrow *v* as mutable because it is also borrowed as immutable." This error occurs because Rust enforces a strict ownership and borrowing model to prevent data races and memory unsafety. In this case, *v4* cannot borrow *v* mutably while *v2* and *v3* still have immutable references to *v*. This is because mutable and immutable references cannot exist simultaneously in Rust to prevent simultaneous modification of data.
